# Supplementary material for: Adversarial Attacks on Black Box Video Classifiers: Leveraging the Power of Geometric Transformations
Source: arXiv:2110.01823 source file (2021-10-26)
Supplement: Supplementary file 1 [file loss_curves_supp.tex]

\begin{figure}[htbp]
	\centering
	\subfloat[Loss curves when using flicker loss.]{
		%\label{fig:Jester_visual}
		\includegraphics[width=0.49\columnwidth]{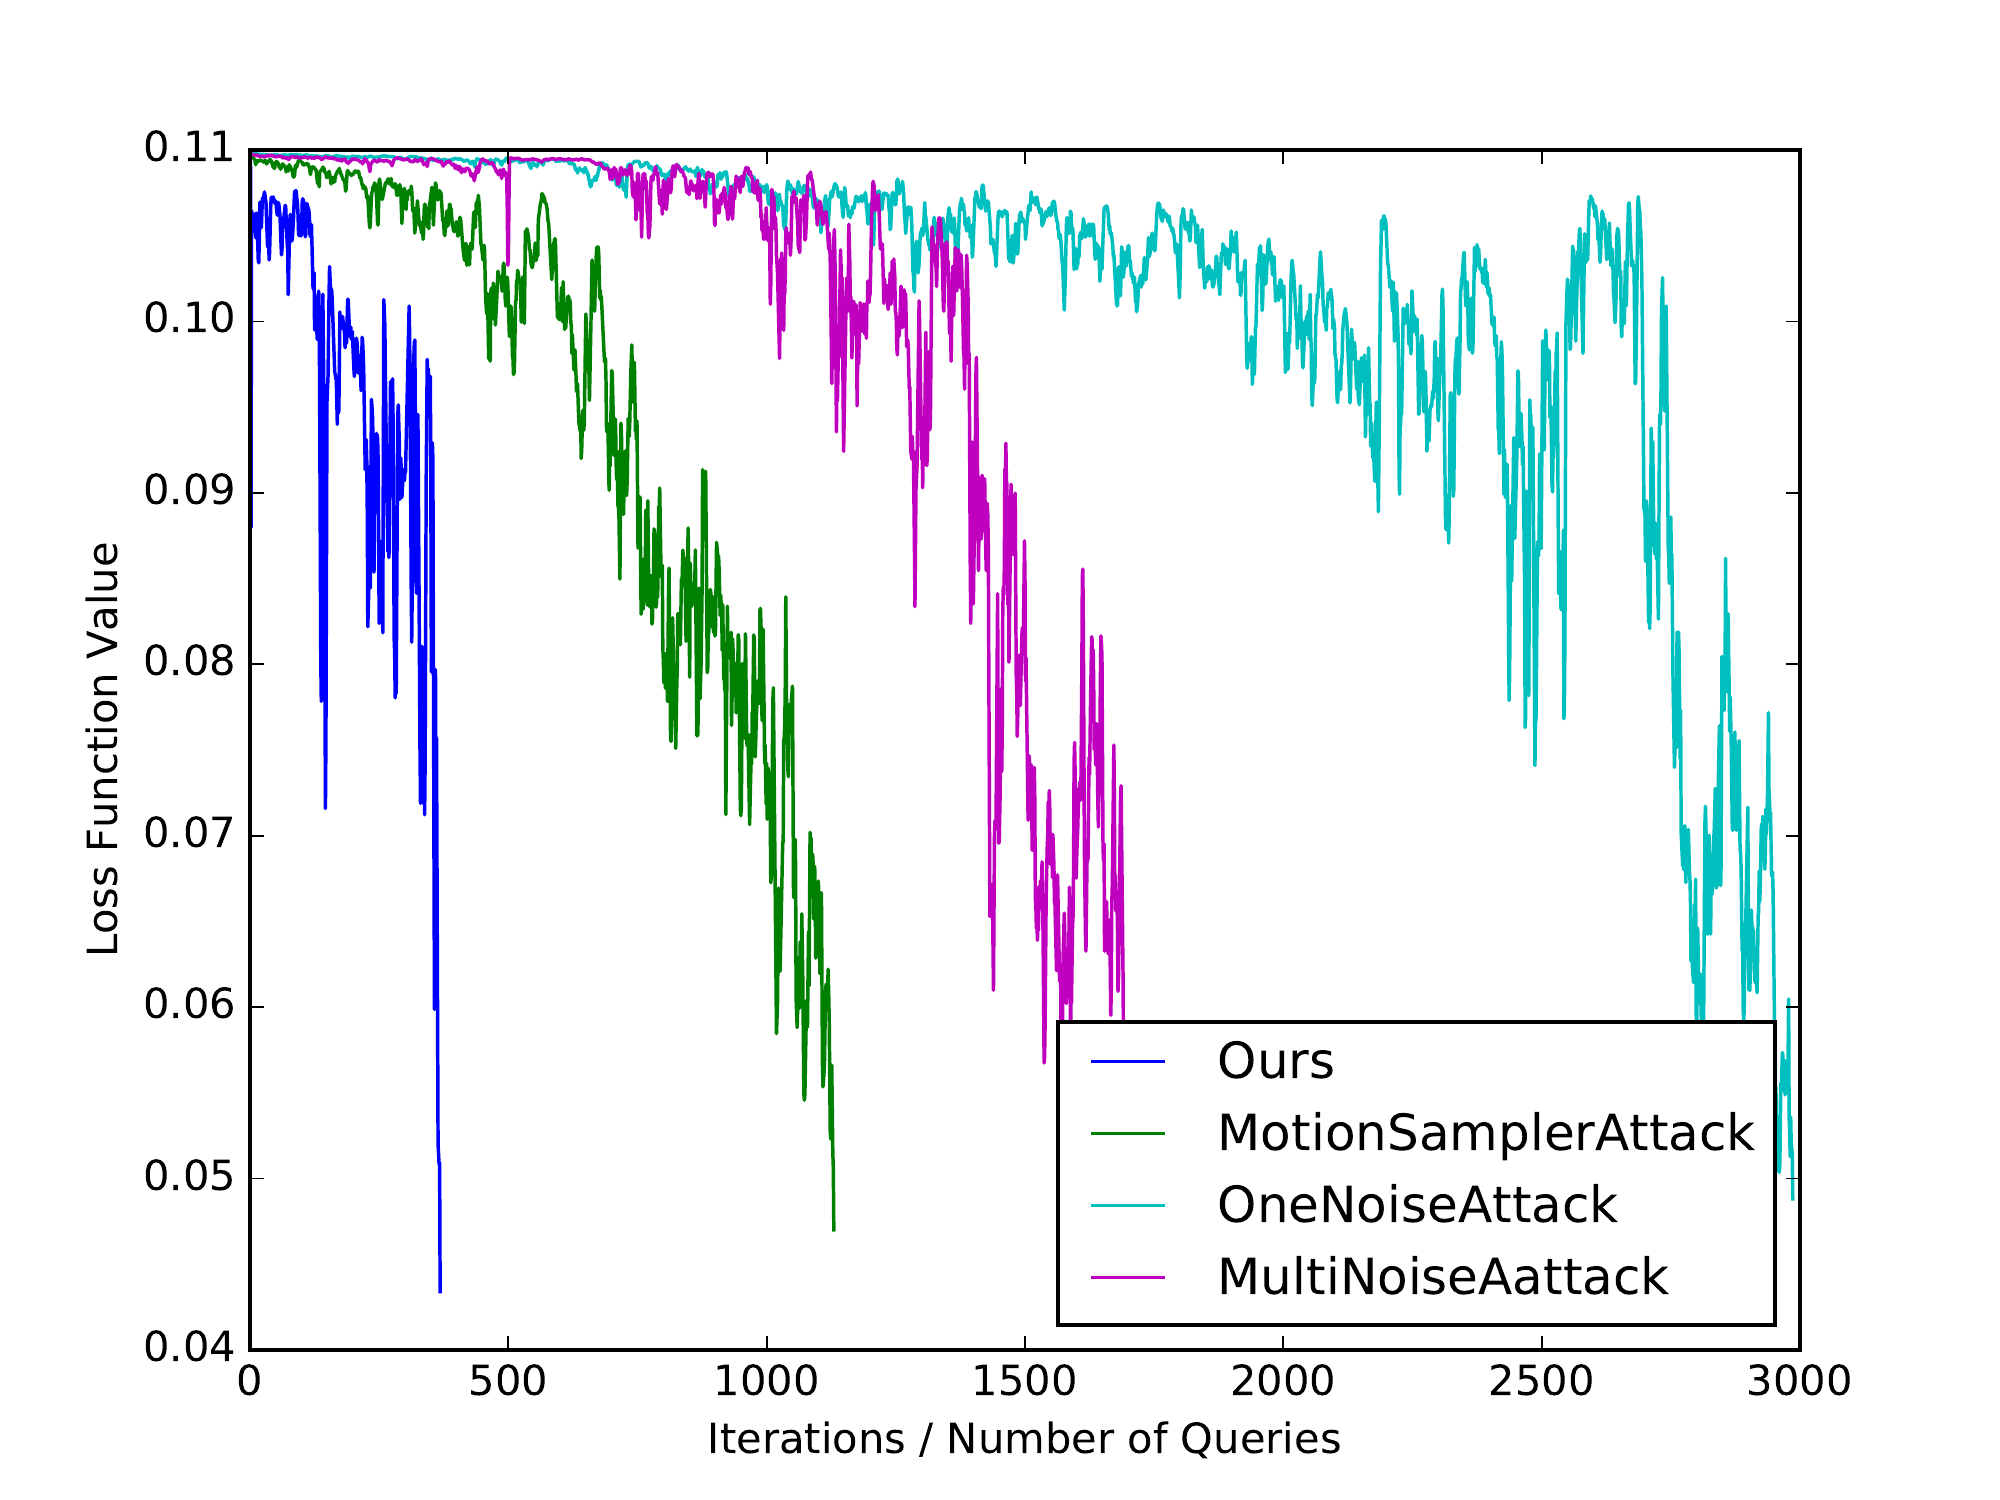} } 
	\subfloat[Gradient magnitude curves when using flicker loss.]{
		%\label{fig:UCF_visual}
		\includegraphics[width=0.49\columnwidth]{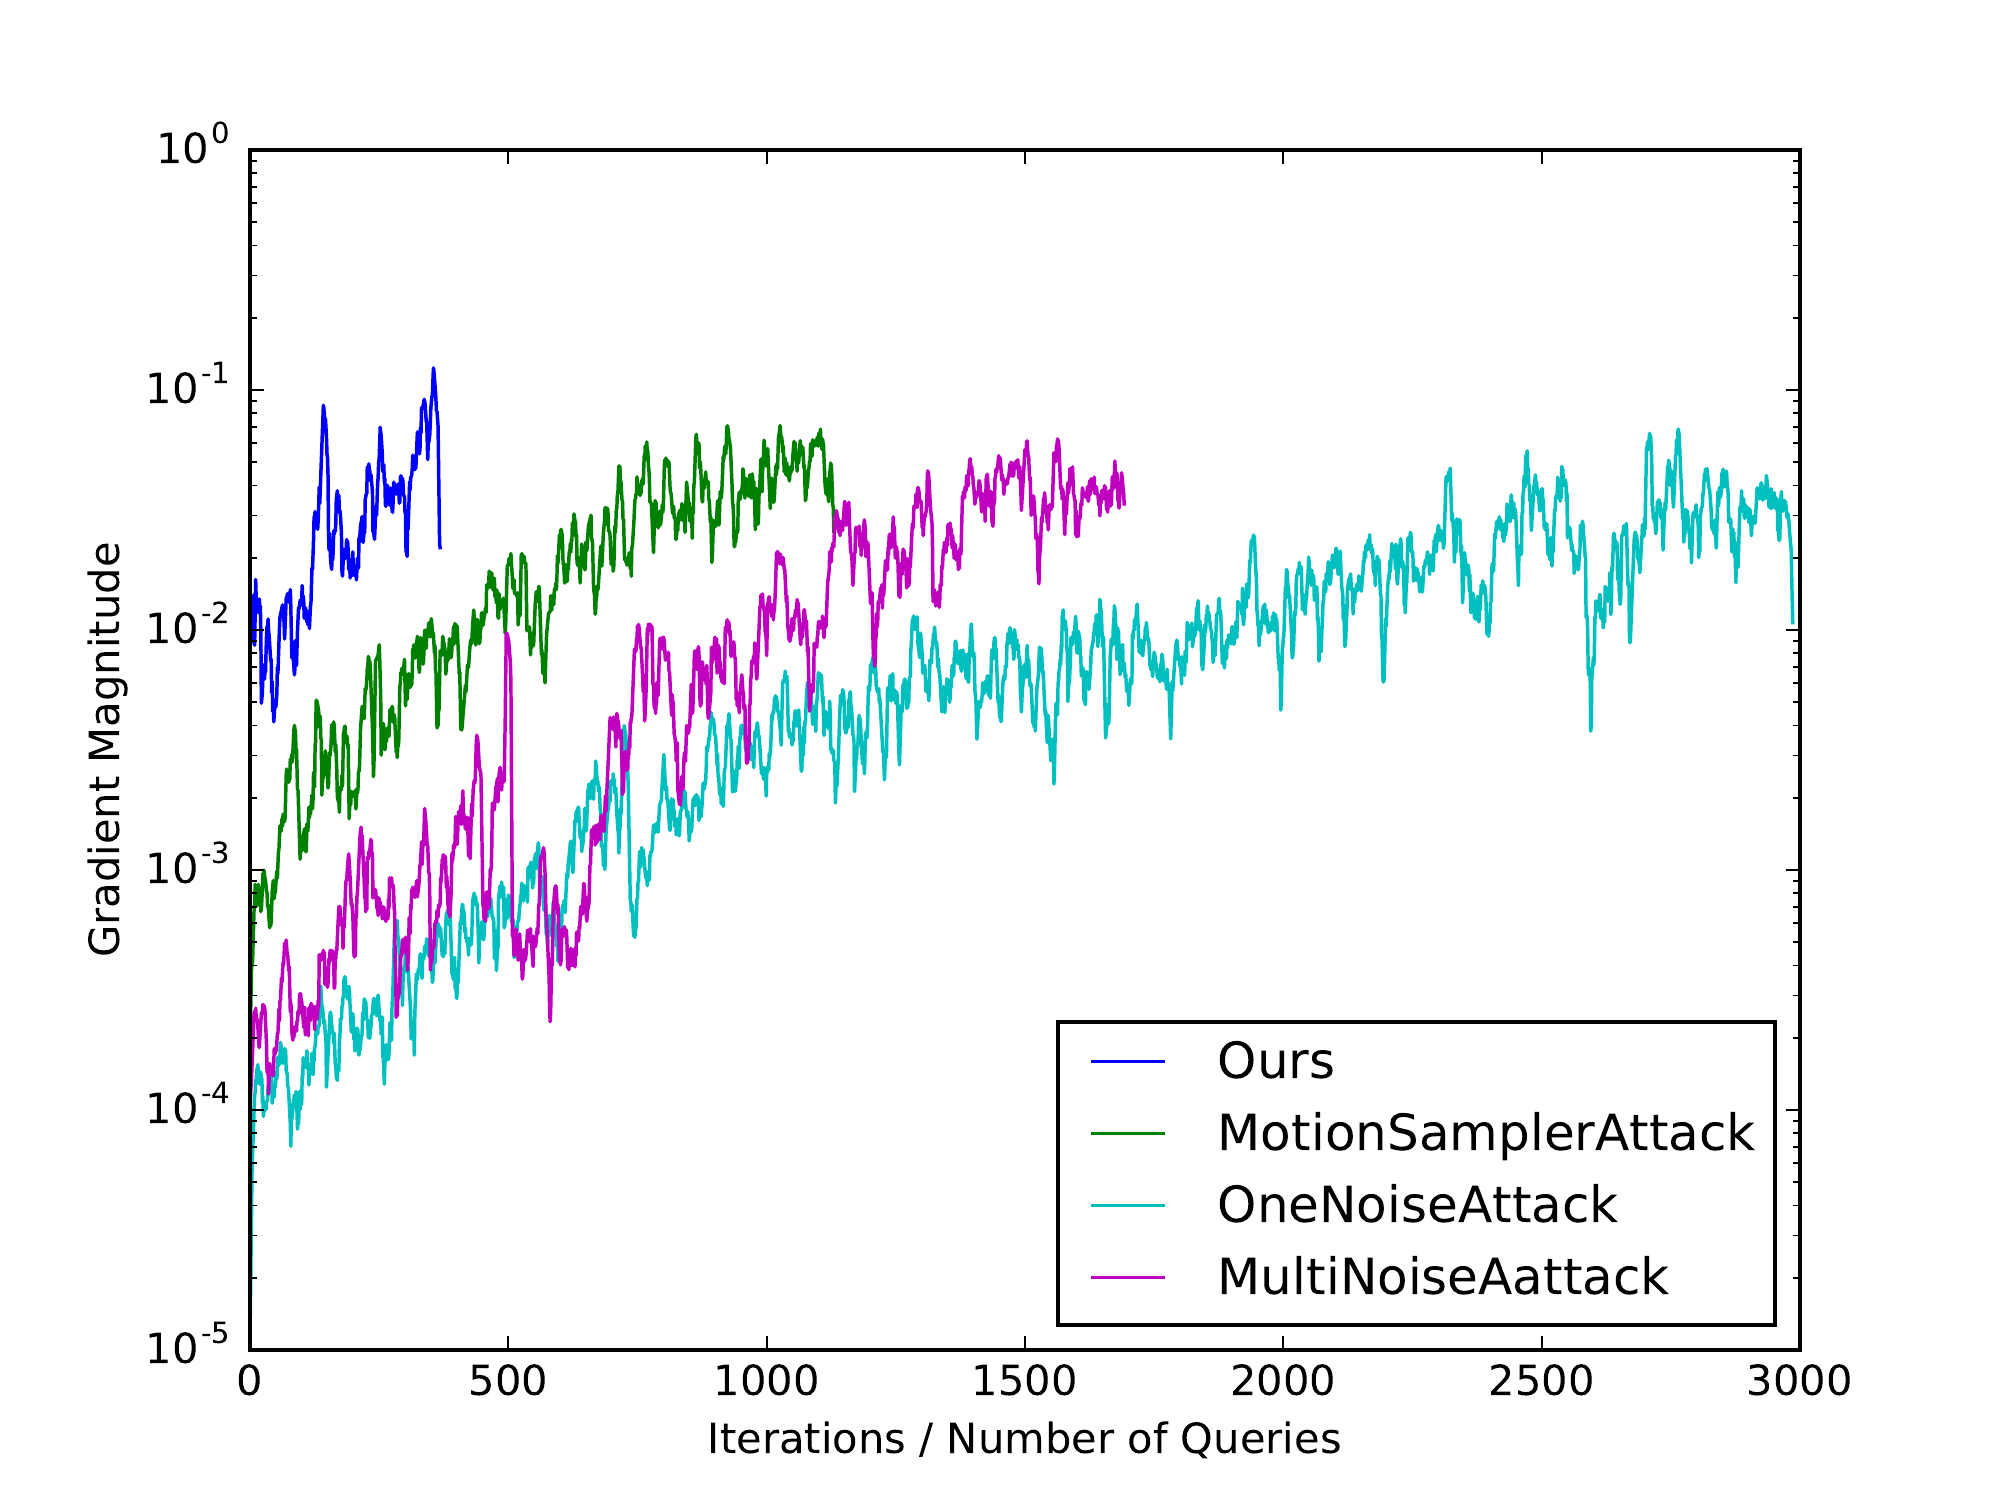} } 
	\\
	\subfloat[Loss curves when using cross entropy loss.]{
		%\label{fig:UCF_visual}
		\includegraphics[width=0.49\columnwidth]{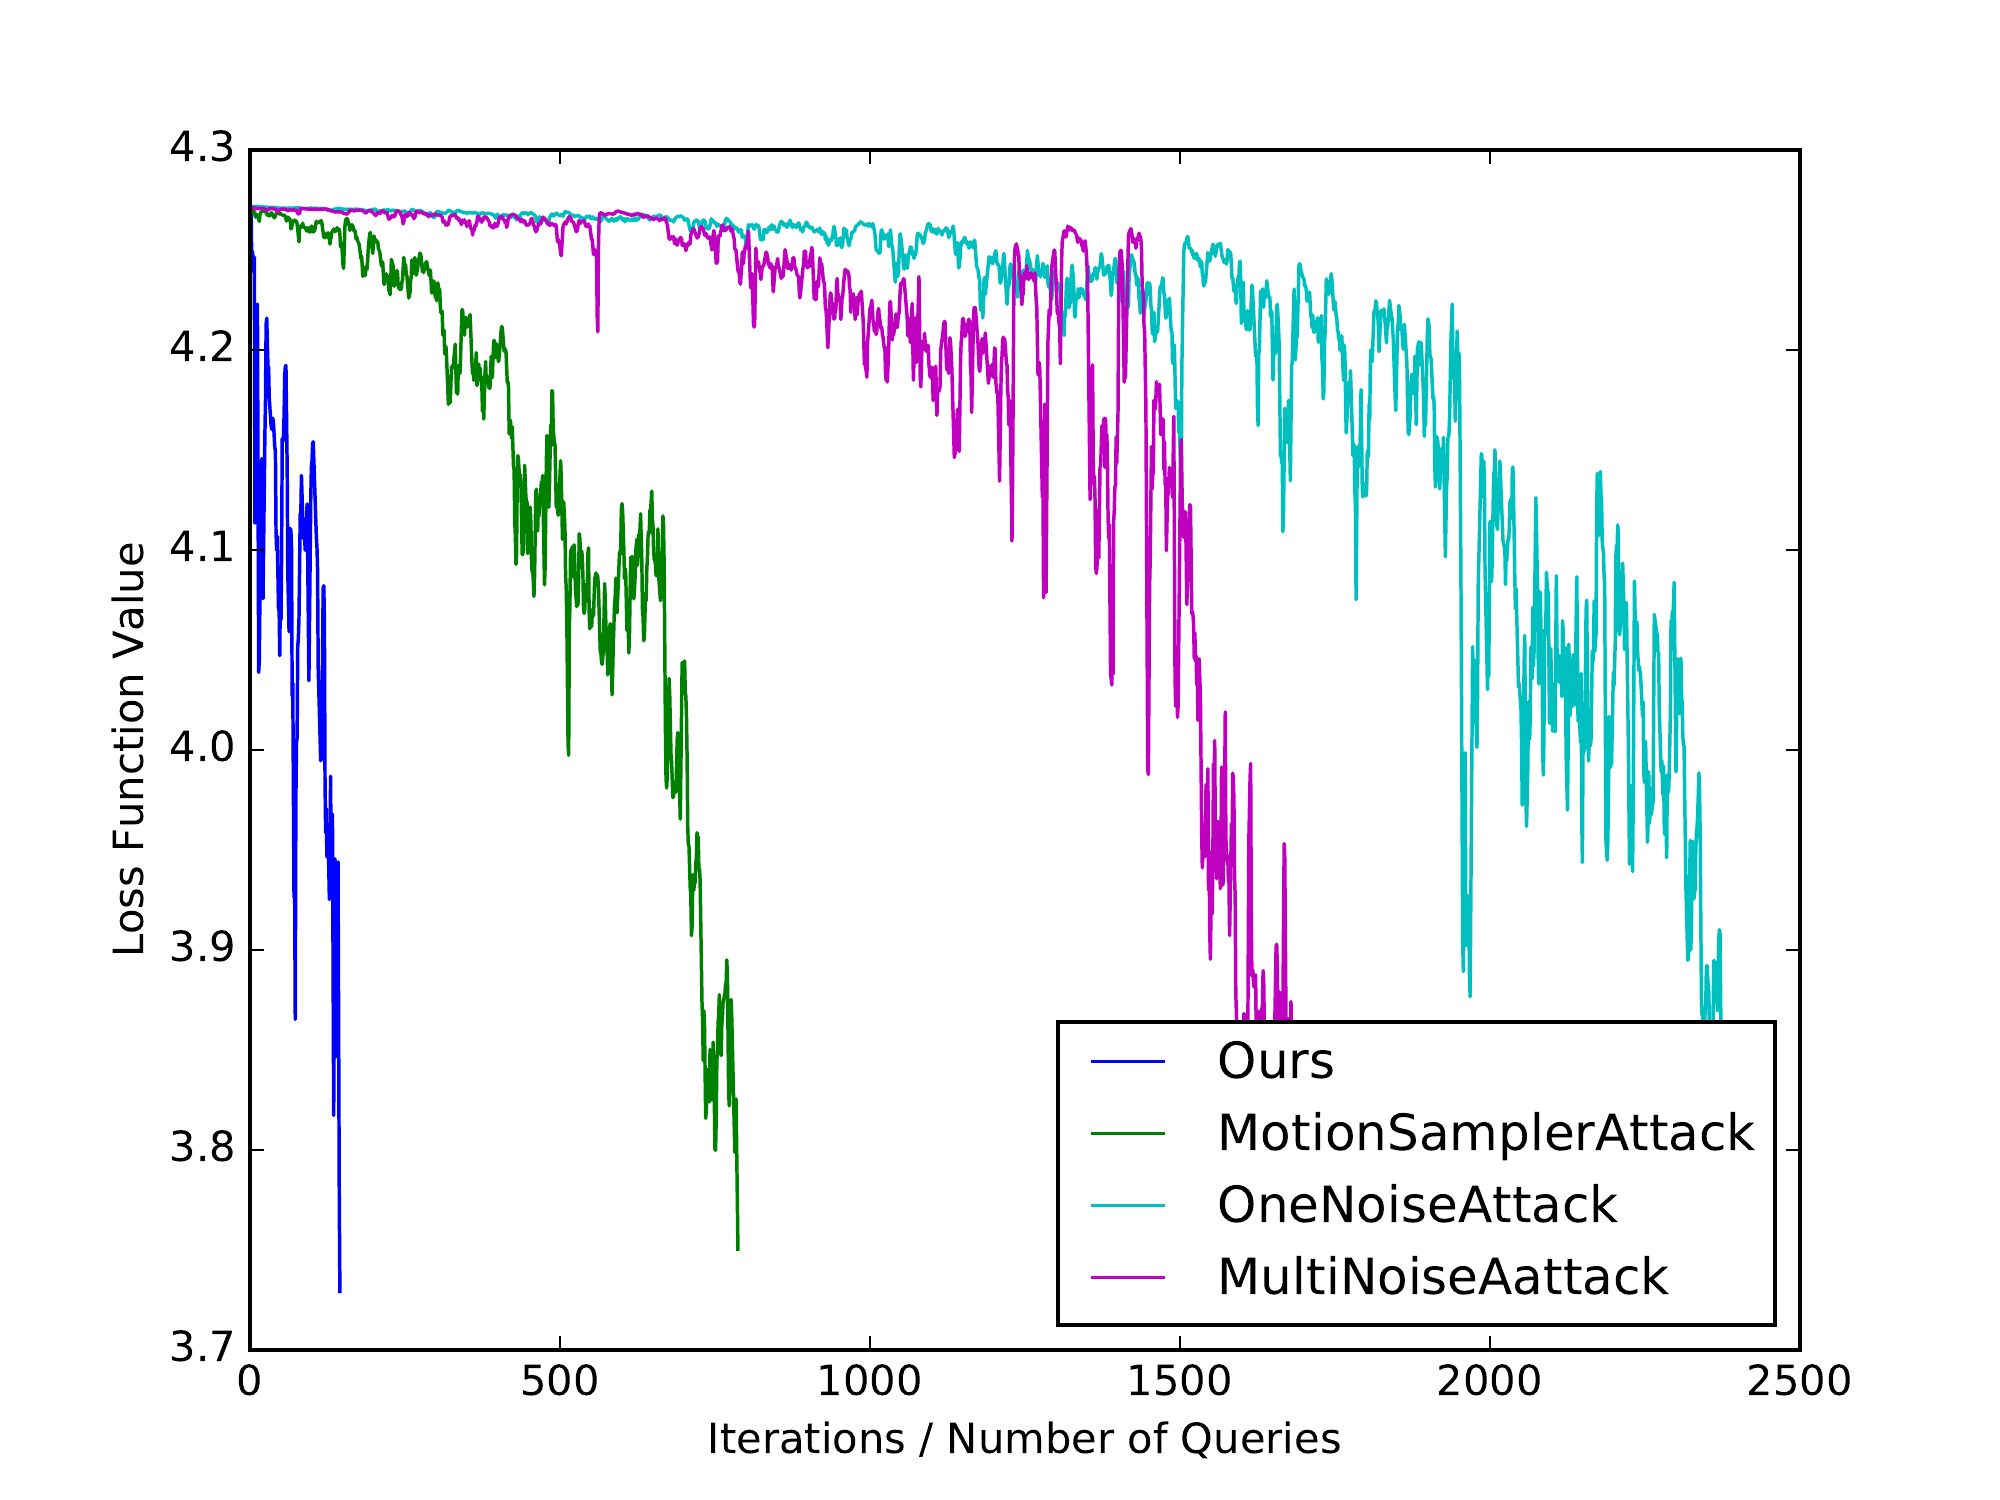} } 
	\subfloat[Gradient magnitude curves when using cross entropy loss.]{
		%\label{fig:UCF_visual}
		\includegraphics[width=0.49\columnwidth]{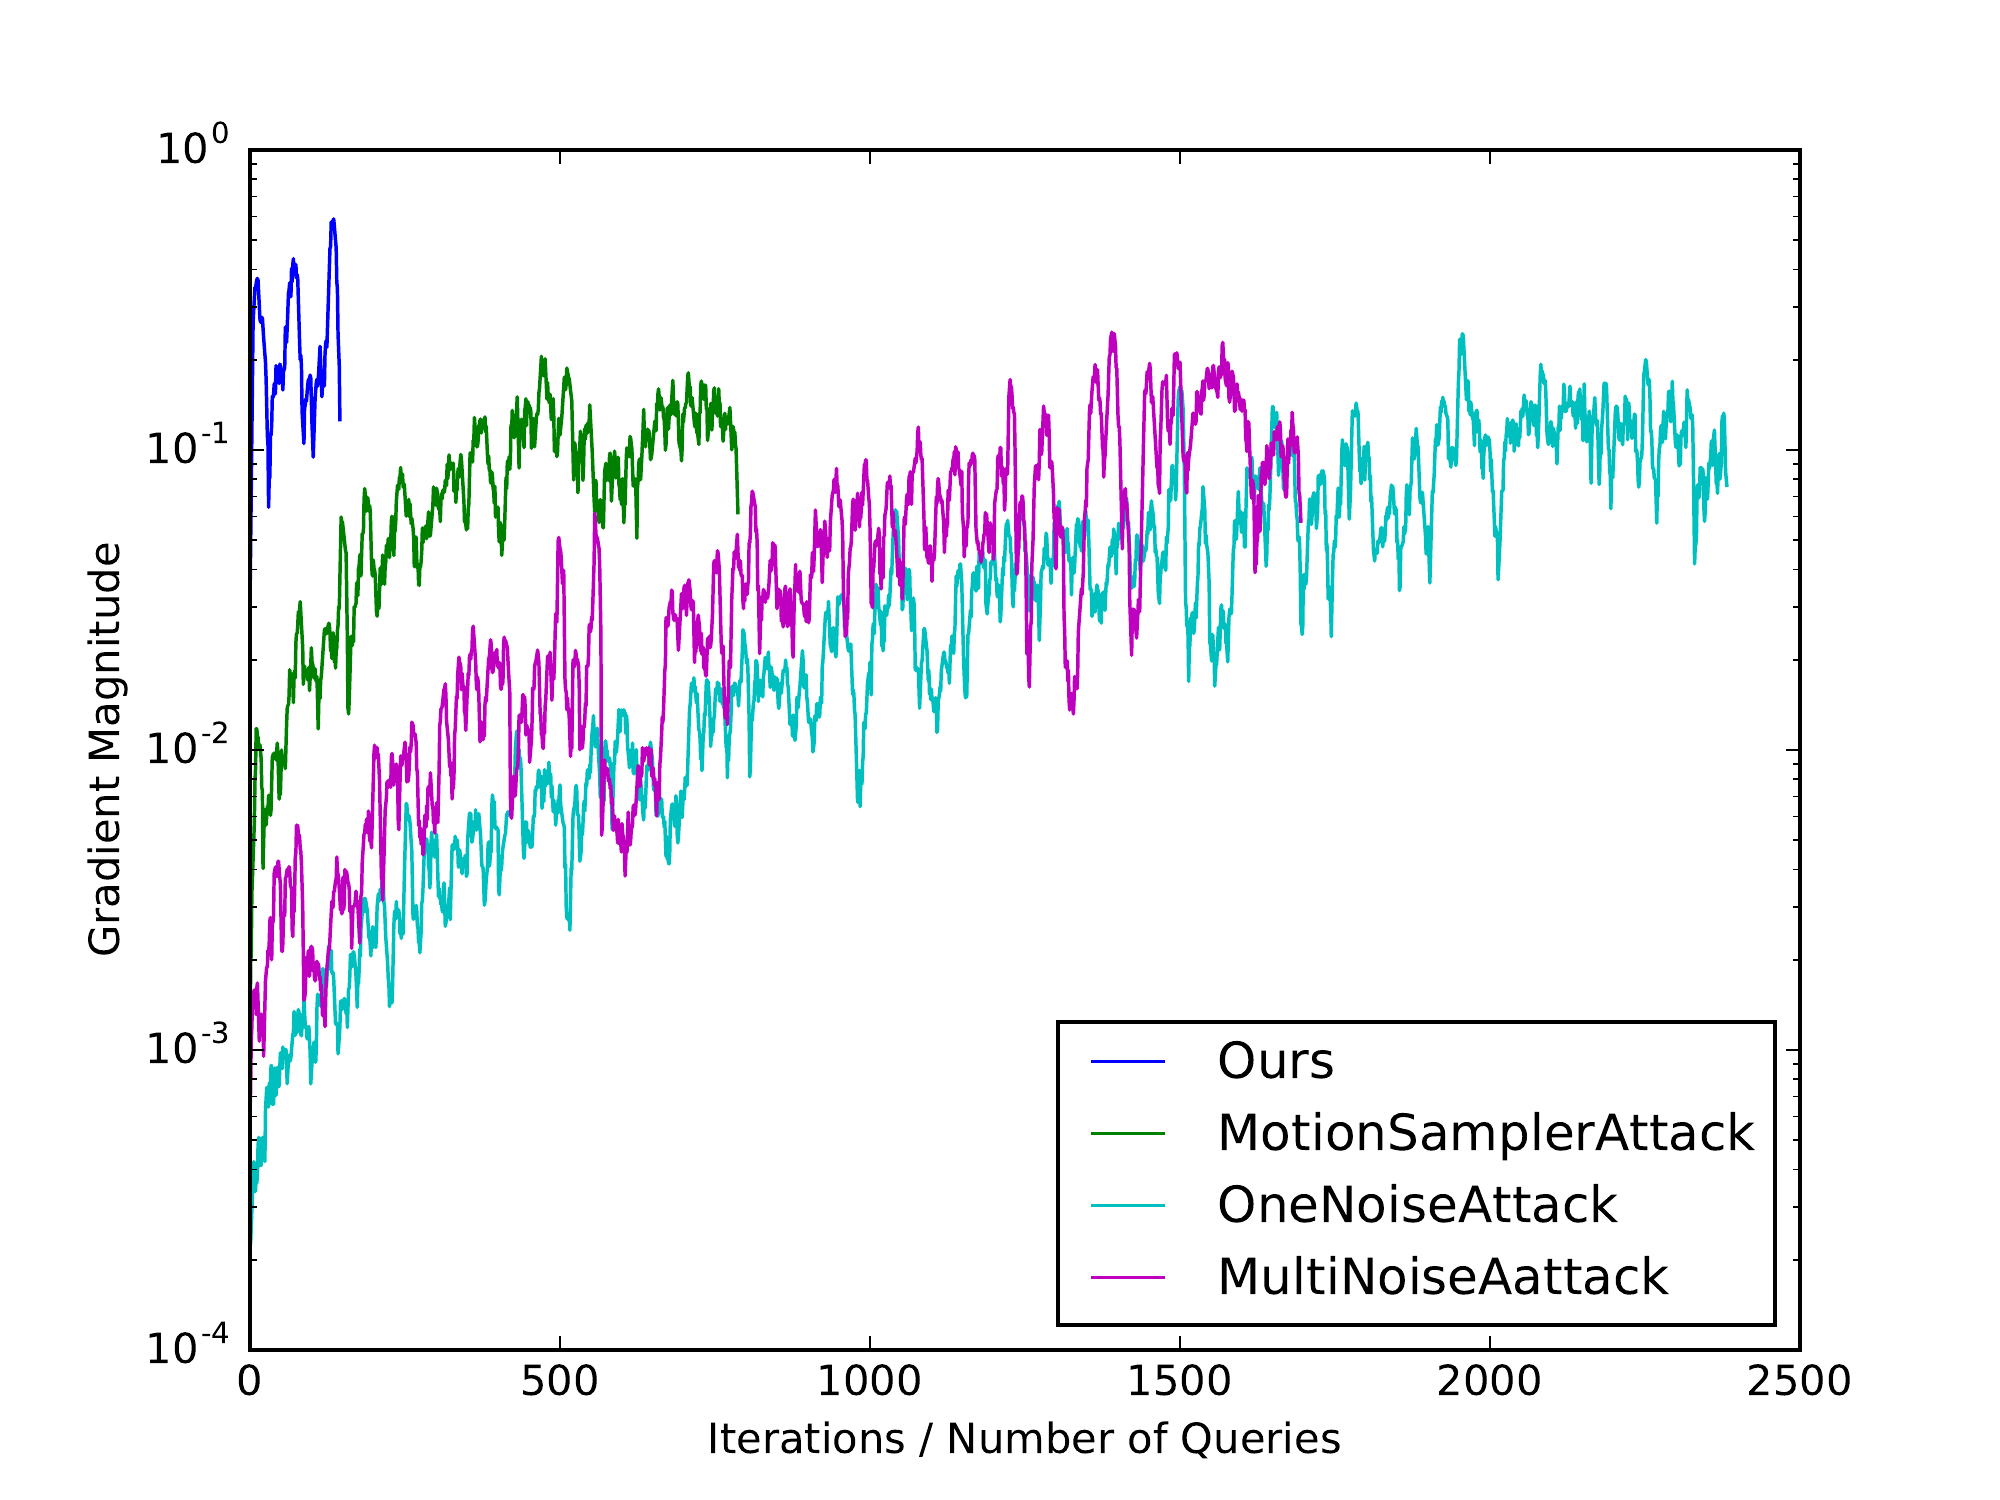} } 
	\\
	\subfloat[Loss curves when using cw2 loss.]{
		%\label{fig:UCF_visual}
		\includegraphics[width=0.49\columnwidth]{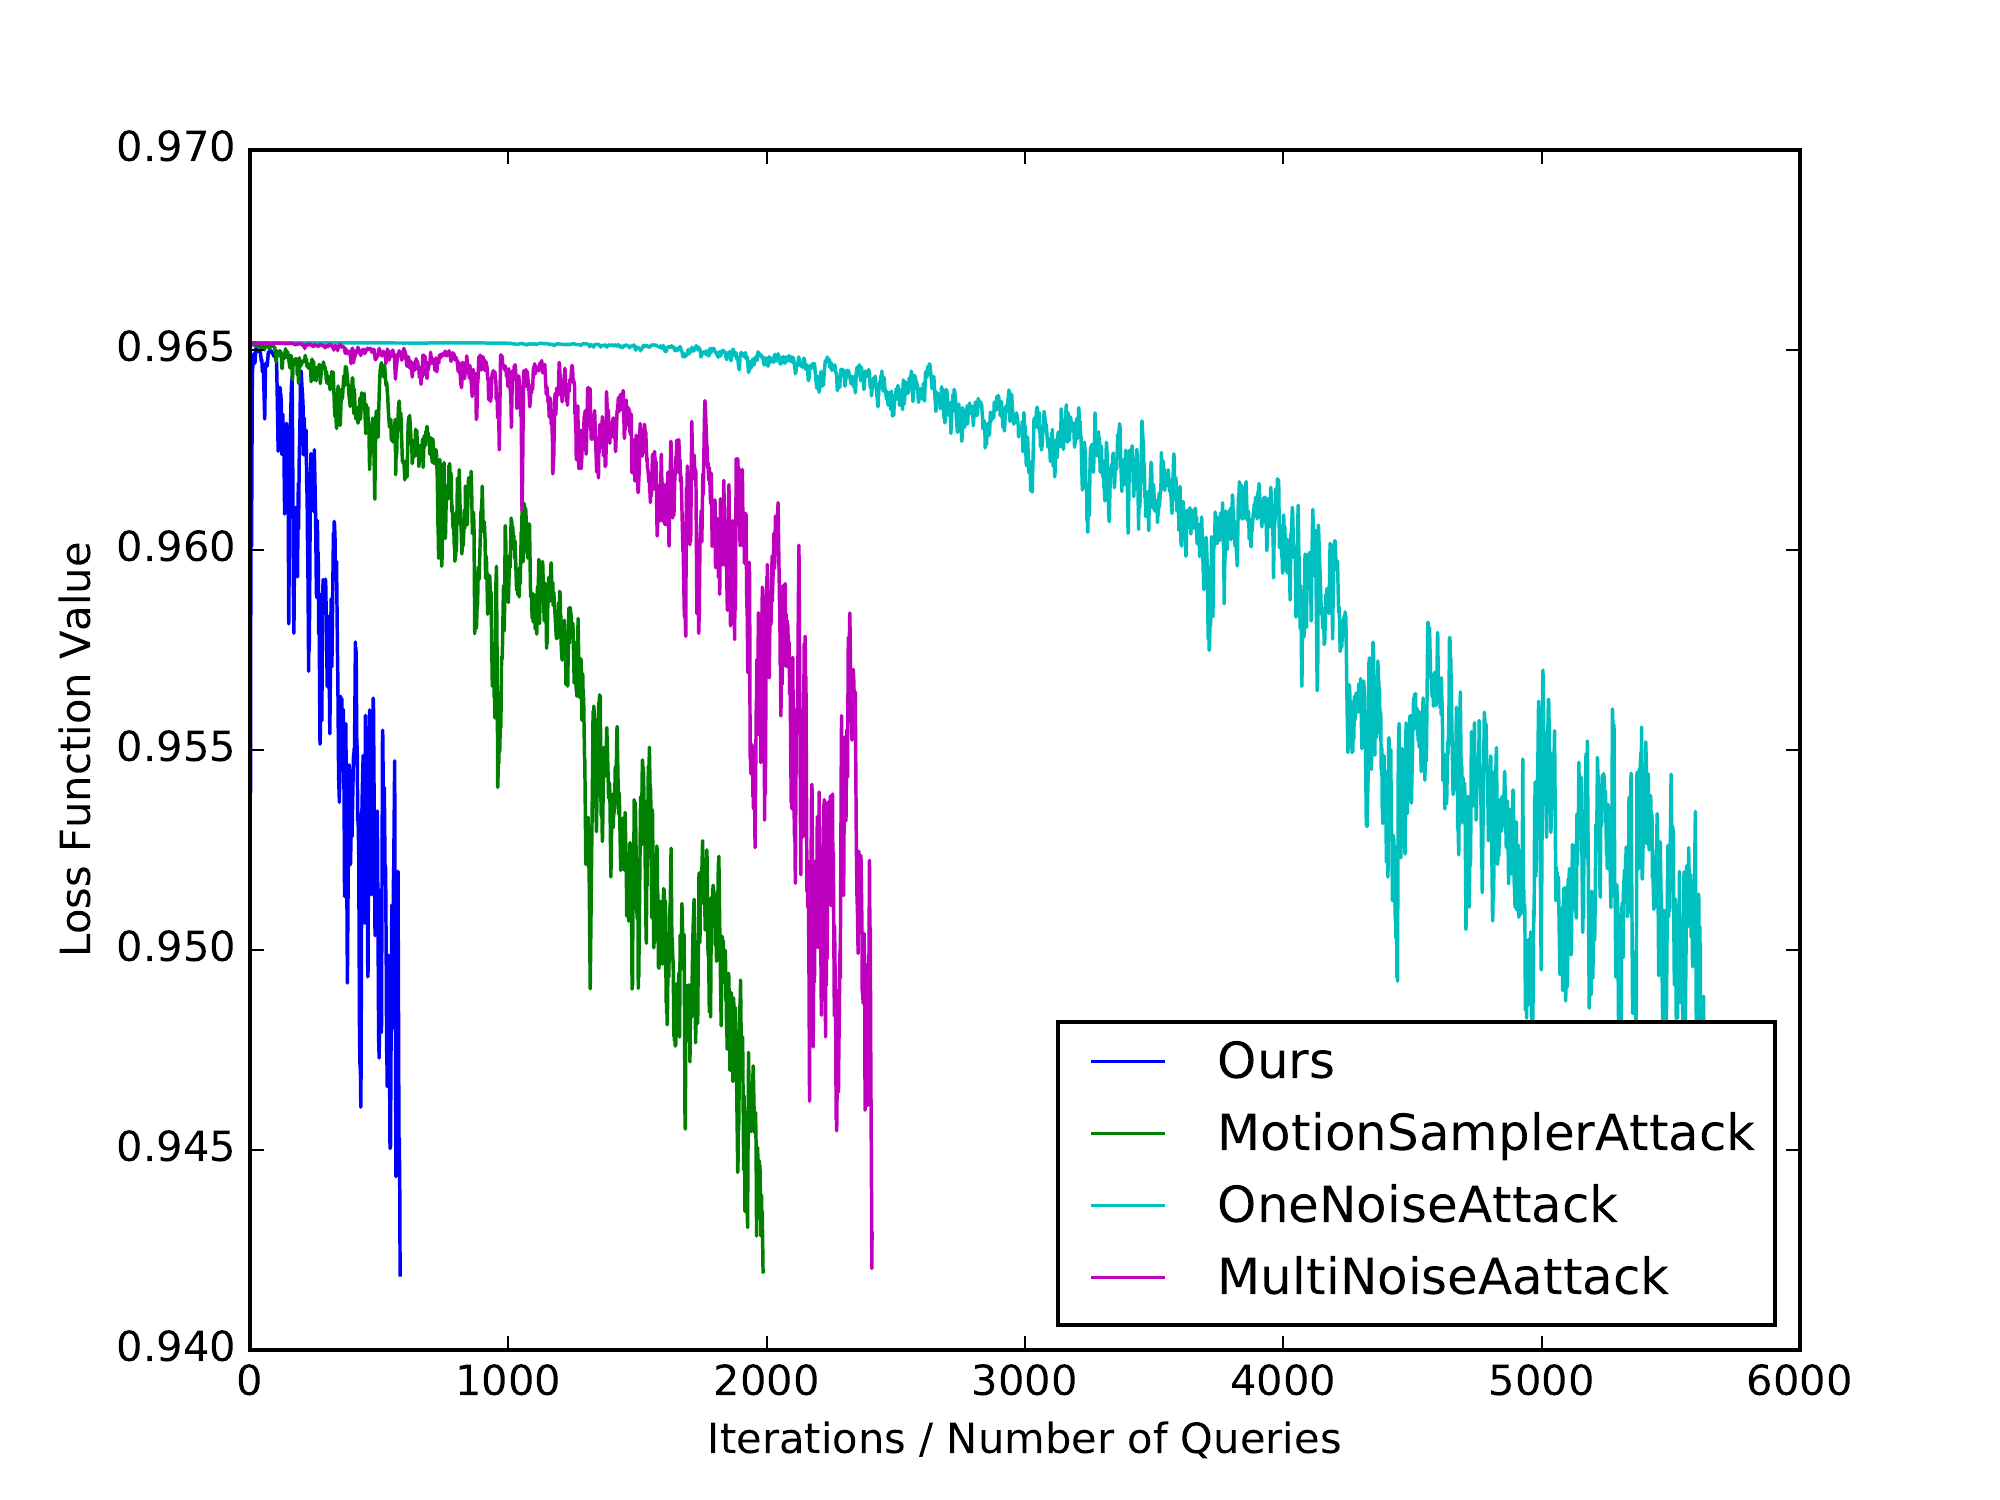} } 
	\subfloat[Gradient magnitude curves when using cw2 loss.]{
		%\label{fig:UCF_visual}
		\includegraphics[width=0.49\columnwidth]{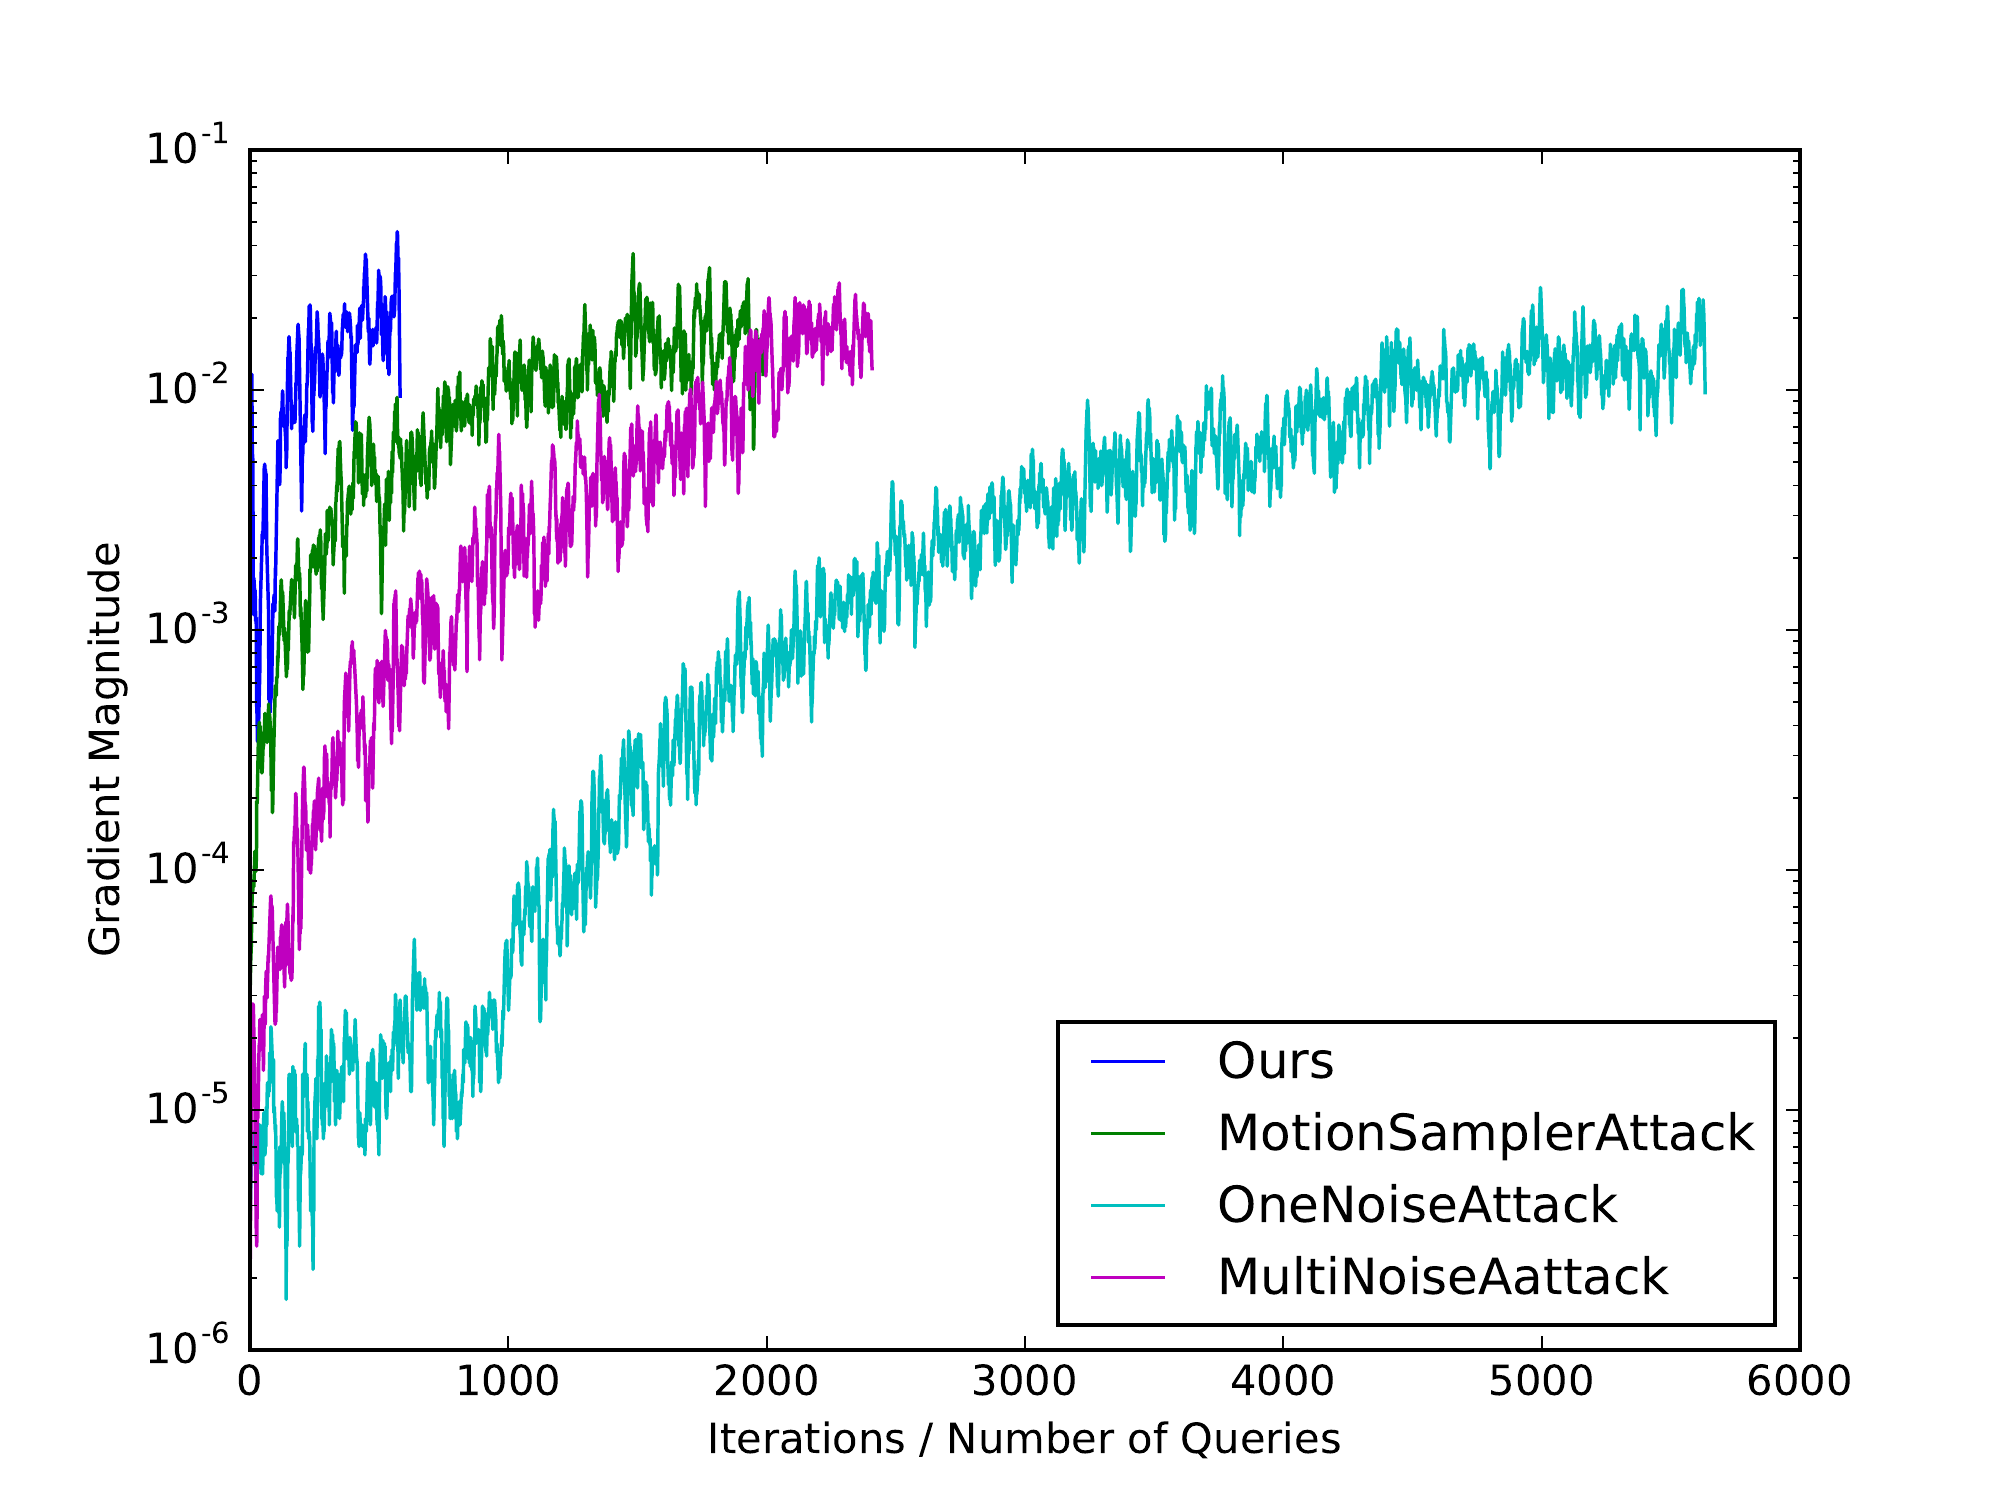} } 
 	\caption{The loss curves and gradient magnitude curves of our method and the three baseline methods when using different loss function.}
	\label{fig:visualization_supp} 
\end{figure}
