# Supplementary material for: Adversarial Attacks on Black Box Video Classifiers: Leveraging the Power of Geometric Transformations
Source: arXiv:2110.01823 source file (2021-10-26)
Supplement: Supplementary file 2 [file cosine_similarity_supp.tex]

\begin{table}[t]
\centering
\caption{Following \cite{jiang2019black}, we evaluate the gradient estimation quality by calculating the cosine similarity between the ground truth gradient $\bm{g}*$ and the estimated gradient $\bm{g}$ calculated by different attack methods. For each dataset, the results (numbers shown in the table * 1e-3) are based on attacks on 1000 randomly chosen videos and the cosine similarity values in the first attack iteration are averaged. We choose the first iteration because the initial $\bm{g}*$  is same for different attack methods. }
\label{tab:cosine_similarity_supp}
%\small
\resizebox{\columnwidth}{!}{
\begin{tabular}{|c|c|c|c|c|c|}
\hline
Dataset                 & Method        & Targeted Aattack & \begin{tabular}[c]{@{}c@{}}Untargeted Attack\\ (flicker loss)\end{tabular} & \begin{tabular}[c]{@{}c@{}}Untargeted Attack\\ (cw2 loss)\end{tabular} & \begin{tabular}[c]{@{}c@{}}Untargeted Attack\\ (cross entropy loss)\end{tabular} \\ \hline
\multirow{4}{*}{Jester} & Ours          & \textbf{2.00}    & \textbf{1.49}                                                              & \textbf{1.38}                                                          & \textbf{1.50}                                                                    \\ \cline{2-6} 
                        & MotionSampler & 1.42             & 1.19                                                                       & 1.04                                                                   & 1.22                                                                             \\ \cline{2-6} 
                        & OneNoise      & 0.83             & 1.06                                                                       & 0.91                                                                   & 1.03                                                                             \\ \cline{2-6} 
                        & MultiNoise    & 0.98             & 0.99                                                                       & 0.88                                                                   & 1.02                                                                             \\ \hline
\multirow{4}{*}{UCF}    & Ours          & \textbf{2.57}    & \textbf{2.36}                                                              & \textbf{2.21}                                                          & \textbf{2.49}                                                                    \\ \cline{2-6} 
                        & MotionSampler & 1.46             & 1.80                                                                       & 1.42                                                                   & 1.66                                                                             \\ \cline{2-6} 
                        & OneNoise      & 0.78             & 0.85                                                                       & 0.68                                                                   & 0.82                                                                             \\ \cline{2-6} 
                        & MultiNoise    & 0.95             & 1.06                                                                       & 0.92                                                                   & 1.01                                                                             \\ \hline
\end{tabular}
}
\end{table}
